# Supplementary material for: Deep Dense Exploration for LLM Reinforcement Learning via Pivot-Driven Resampling
Source: arXiv:2602.14169 source file (2026-06-12)
Supplement: Supplementary file 1 [file limitations_and_futurework.tex]

\section{Limitations and Future Work}
\label{app:limitations_future_work}

While DEEP-GRPO demonstrates significant improvements in reasoning performance, we acknowledge certain limitations in its current implementation and outline potential directions for future research.

\paragraph{Computational Overhead and Throughput.}
A primary limitation of DEEP-GRPO is the additional computational overhead introduced by its two-stage sampling mechanism. Compared to GRPO, which maximizes throughput via parallel root sampling, our method requires re-initiating generation from intermediate pivots. This sequential dependency reduces the overall training speed.

\paragraph{Exploration Efficiency on Hard States.}
Despite utilizing the depth bias ($\gamma$) to guide exploration towards deep, error-prone states, we observe that a significant fraction of these selected pivots still fail to yield a correct solution. As illustrated in Figure~\ref{fig:unrecoverable_states}, the number of ``unrecoverable'' states—where dense resampling fails to find any correct path—remains non-negligible throughout training. This suggests that for certain deep states containing errors, simple rejection sampling may not suffice to recover the correct reasoning path.

\begin{figure}[ht]
    \centering
    \includegraphics[width=\linewidth]{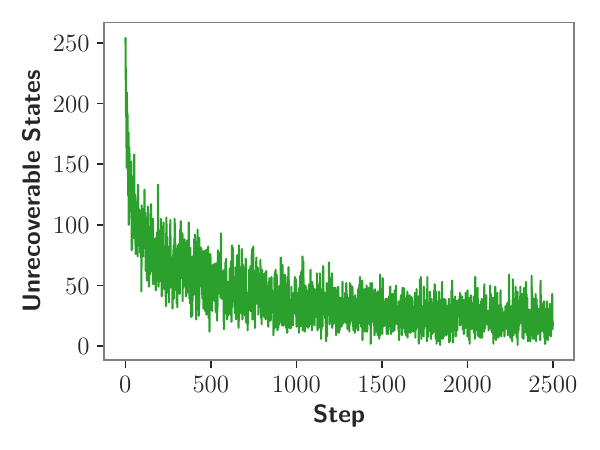} 
    \caption{Analysis of Exploration Success Rate. The curve shows the number of pivot states where dense exploration failed to recover a correct solution during training. Despite our targeted strategy, a substantial portion of deep error states remain unrecoverable, indicating the difficulty of self-correction in sparse reward environments.}
    \label{fig:unrecoverable_states}
\end{figure}

\paragraph{Future Work.}
To address these challenges, we plan to explore the following directions:
\begin{itemize}
    \item Deferred Branching Mechanism: To mitigate the latency of the two-stage process, we aim to unify the exploration into a single-stage framework. Drawing inspiration from AttnRL~\cite{liu2025attention}, we aim to unify the exploration into a more efficient pipeline. Instead of performing immediate branching which interrupts the generation flow, we plan to collect identified pivot states and incorporate them as prefixes into subsequent training batches. This approach allows for continuous generation without the "pause-and-resample" overhead, effectively treating intermediate state exploration as a form of dynamic prompt augmentation within the standard data stream.
    \item Synthetic Data from Hard Failures: To address the issue of unrecoverable states, we propose to utilize the ``hard'' states collected during failed exploration attempts. Rather than discarding these states, we plan to use them as seeds for generating synthetic data—potentially leveraging stronger teacher models or more computationally intensive search methods (e.g., MCTS) to find solutions offline. These synthesized trajectories can then be used for Supervised Fine-Tuning (SFT), effectively turning current exploration failures into high-value training signals for future iterations.
\end{itemize}
